# Supplementary material for: RSCFed: Random Sampling Consensus Federated Semi-supervised Learning
Source: arXiv:2203.13993 source file (2022-03-26)
Supplement: Supplementary file 1 [file Supp.tex]

\appendix

\section{Ablation Study for Various Unlabeled Client Ratios when Partitioning Fixed}

We demonstrate that the effectiveness of our RSCFed is \textbf{\emph{due to uneven model reliability caused by the involved unlabeled clients.}} With a fixed number of clients, the more unlabeled clients, the better our RSCFed is. 

% We perform an ablation study towards unlabeled clients ratio to elaborate its relevance with RSCFed's effectiveness when data partitioning is fixed.

Fig.~\ref{supp} shows the performance of our method and the baseline method Fed-Consist~\cite{yang2021federated} under different labeled and unlabeled client ratios.   
%The experiment is conducted with a fixed number of clients and different ratios of engaging unlabeled clients, and we compare the performance of Fed-Consist~\cite{yang2021federated} and RSCFed in Accuracy and AUC score. 
We empirically set the number of clients to 10 and consider the ratio of unlabeled/total clients as 0, 0.4, 0.6, 0.7, 0.8, 0.9.

We can observe that as the ratio of unlabeled clients increases, the improvements of our RSCFed over Fed-Consist in Accuracy and AUC scores consistently grow. 
It is worth mentioning that when the unlabeled ratio is small, a slight performance drop can be observed from our RSCFed against Fed-Consist. This is because the increased number of labeled clients reduce the \emph{uneven model reliability}, limiting the performance of our RSCFed.
Notably, RSCFed exceeds Fed-Consist when the ratio of unlabeled clients comes to 0.7.  When the unlabeled ratio is 0.9, our RSCFed can reach 3.32\% and 1.31\% improvements in Accuracy, and AUC scores, respectively.  %when unlabeled clients take 0.9. 
%
%Improvements in both metrics progressively increase with the growth of unlabeled clients ratio. 
Therefore, we demonstrate that with a fixed number of clients, the more unlabeled clients involved, the better our RSCFed is.

%as the total number of clients is fixed to 10, it can be proved that the effectiveness of our method lies only with the increase of unlabeled clients ratio.

\begin{figure}[!h]
\centering
    \includegraphics[width=\linewidth]{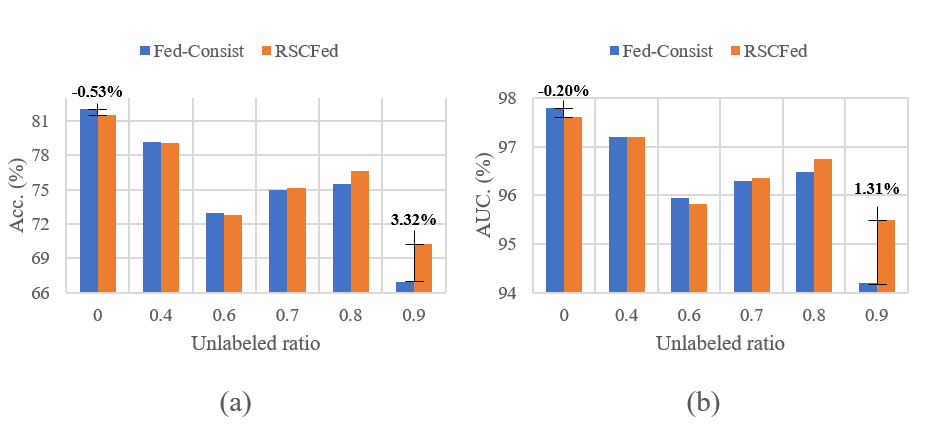}
    \caption{Performance curve of Fed-Consist~\cite{yang2021federated} and our RSCFed under various unlabeled client ratios. The total number of clients is fixed to 10, and the $x$-axis refers to ratio of unlabeled clients among all clients.} 
    \label{supp}
    %\vskip -15pt
\end{figure}

\section{Implementation Details}
\noindent
All local training in RSCFed is implemented with an SGD optimizer. The local learning rate is set according to the dataset. Specifically, for the SVHN dataset and CIFAR-100 dataset, we set the learning rate to 0.03 and 0.021 for labeled and unlabeled clients, respectively; For ISIC 2018 dataset, we set the learning rate to 2e-3 and 1e-3 for labeled and unlabeled clients, respectively. In each synchronization round, after the first global model is randomly initialized and assigned to the client-side, we firstly conduct supervised local training on the labeled client for six local epochs as a warming-up. The supervised pre-heated model then serves as the global model for training on labeled and unlabeled clients. In total, we train the model for 1,000 synchronization rounds~\footnote{We will release our code and trained models at GitHub upon acceptance}.
